# Supplementary material for: Next-to-next-to-leading order event generation for top-quark pair production
Source: arXiv:2012.14267 source file (2022-02-24)
Supplement: Supplementary file 1 [file all_plots_paper_supplemental.pdf]

$pp \rightarrow t\bar{t}$  @ 13 TeV

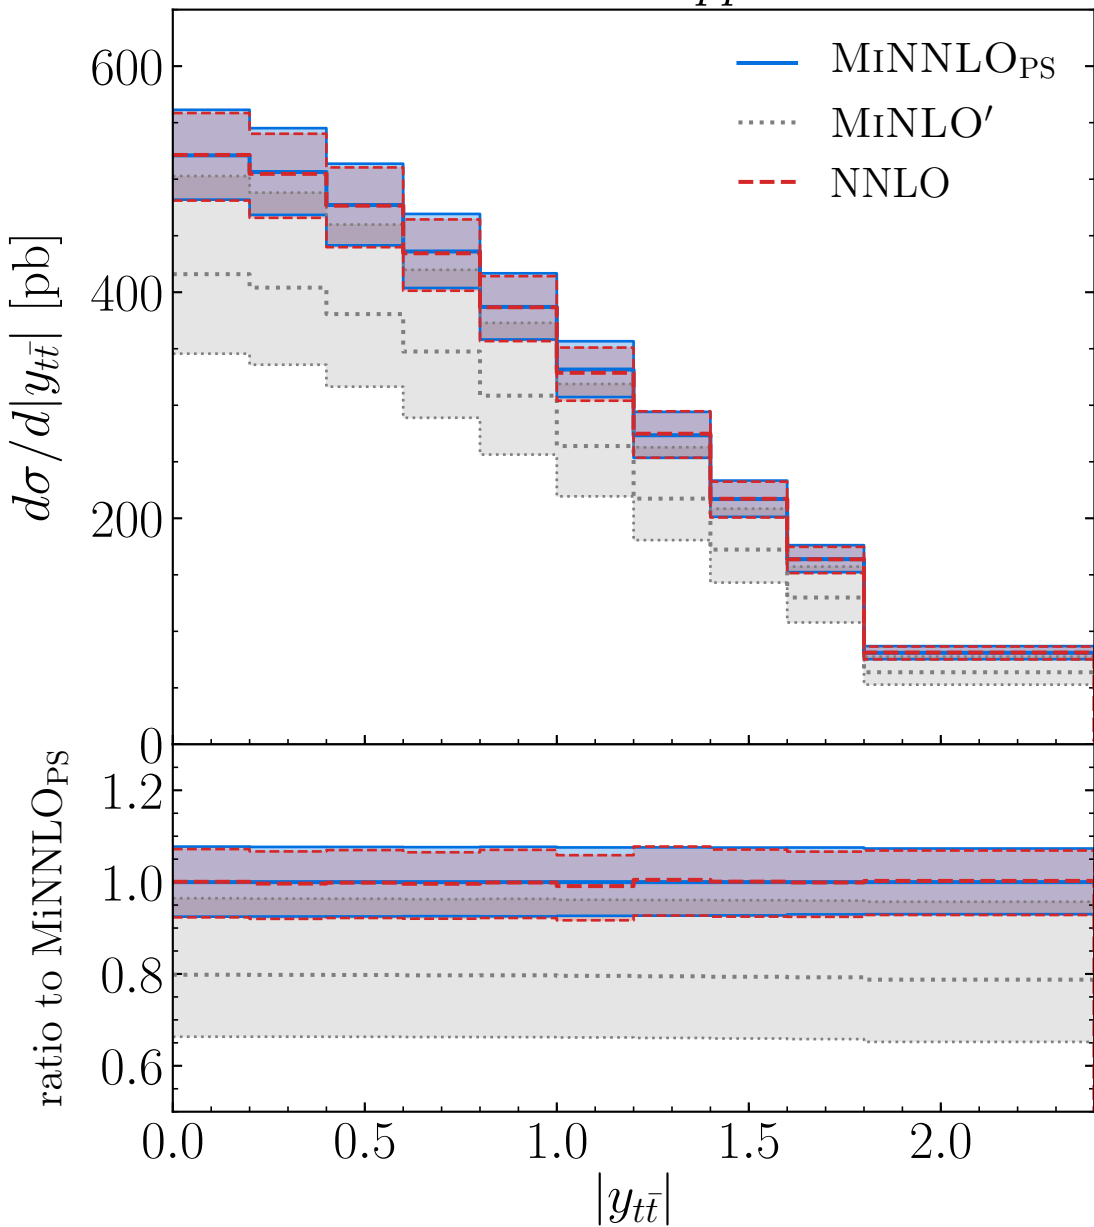

$pp \rightarrow t\bar{t}$  @ 13 TeV

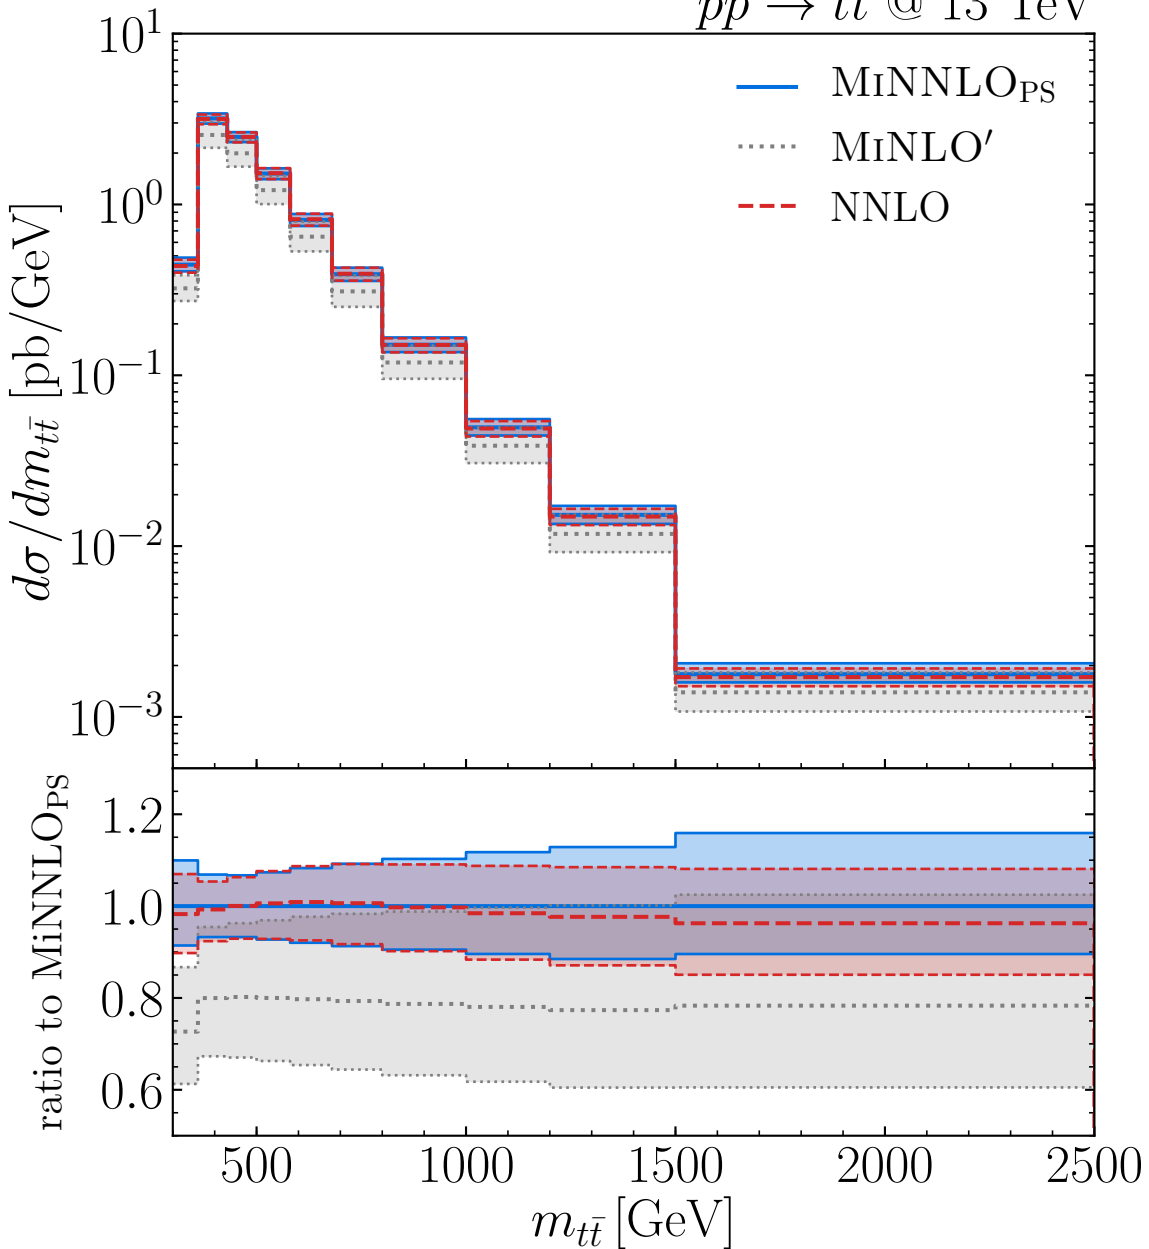

$pp \rightarrow t\bar{t}$  @ 13 TeV

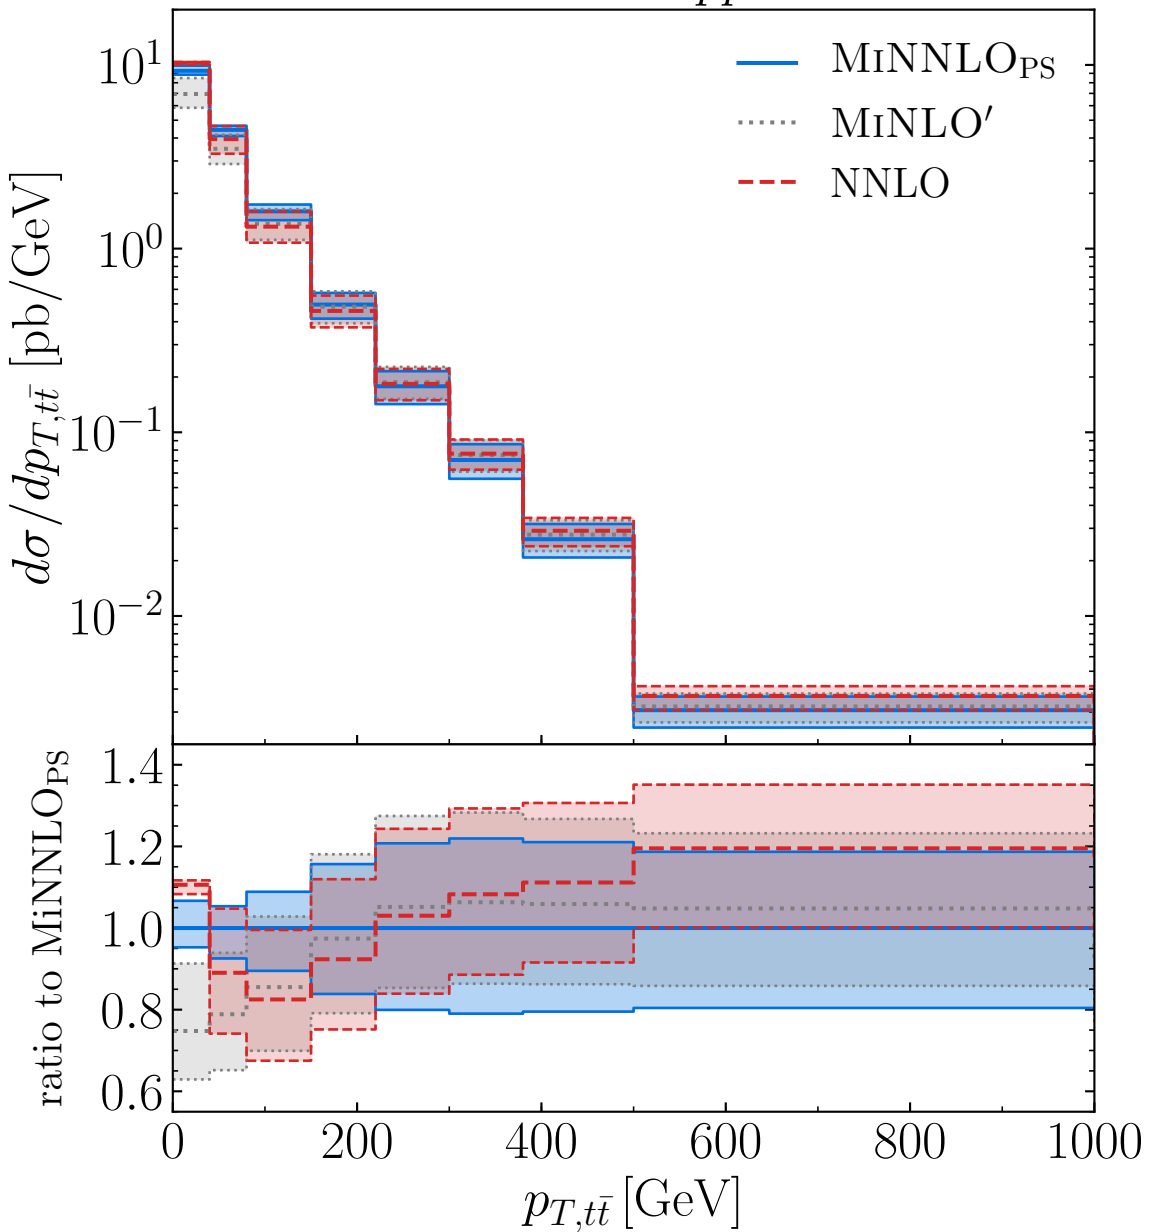

$pp \rightarrow t\bar{t}$  @ 13 TeV

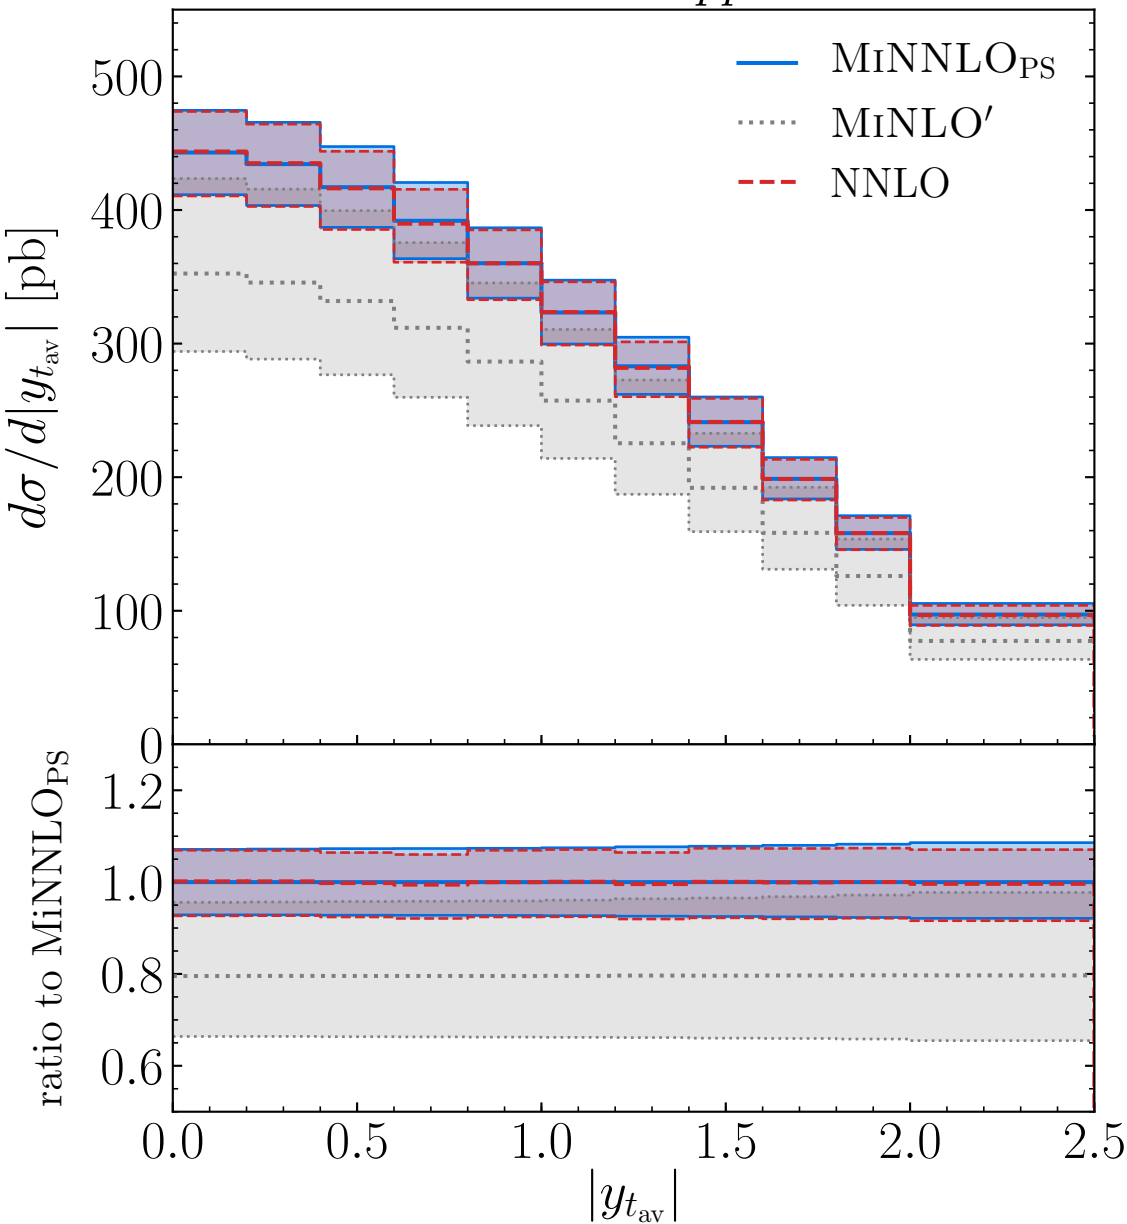

$pp \rightarrow t\bar{t}$  @ 13 TeV

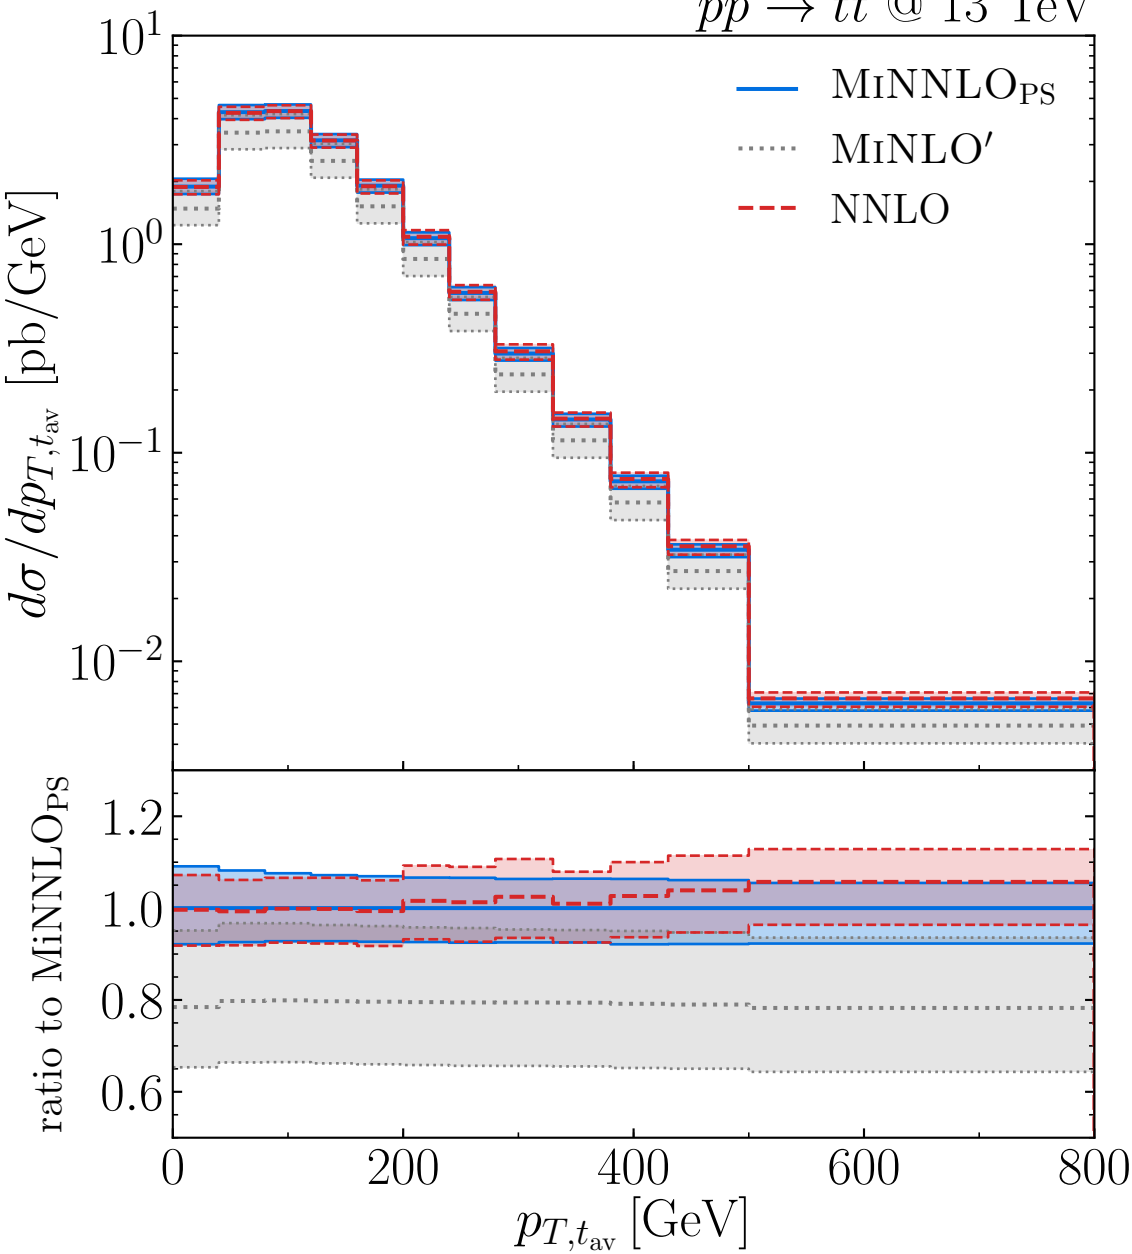

$pp \rightarrow t\bar{t}$  @ 13 TeV

$p_{T,j_1} > 120$  GeV

$d\sigma/d\Delta y_{t\bar{t},j_1}$  [pb]

— MiNNLO<sub>PS</sub>  
... MiNLO'

ratio to MiNNLO<sub>PS</sub>

1.2  
1.0  
0.8

$\Delta y_{t\bar{t},j_1}$

4

2

0

-2

-4
